# Supplementary material for: Bind-Your-Avatar: Multi-Talking-Character Video Generation with Dynamic 3D-mask-based Embedding Router
Source: arXiv:2506.19833 source file (2025-06-24)
Supplement: Supplementary file 1 [file X_suppl.tex]

% \clearpage
% \setcounter{page}{1}
% \maketitlesupplementary
